# Supplementary material for: Automatic Selection of t-SNE Perplexity
Source: arXiv:1708.03229 source file (2017-08-10)
Supplement: Supplementary file 1 [file appendix.tex]

\section*{Appendix}
\label{appendix}
In this section, we present additional experiments on three more datasets, but comparing to preferences collected from a single human expert. The three datasets are Image Segmentation\footnote{\tiny{https://archive.ics.uci.edu/ml/datasets/Image+Segmentation}}, Cardiotocography \footnote{\tiny{https://archive.ics.uci.edu/ml/datasets/Cardiotocography}}, and Abalone dataset\footnote{\tiny{https://archive.ics.uci.edu/ml/datasets/Abalone}}. The Image Segmentation data set contains 2310 points, while the Cardiotocography and Abalone data have 2126 instances and 4177 points, respectively. For each experiment, 100 user preferences are collected.

\begin{figure}[h]
  \centering
  \begin{subfigure}{\label{fig:image_seg_cl}}
      \centering
  \includegraphics[width=2.6in]{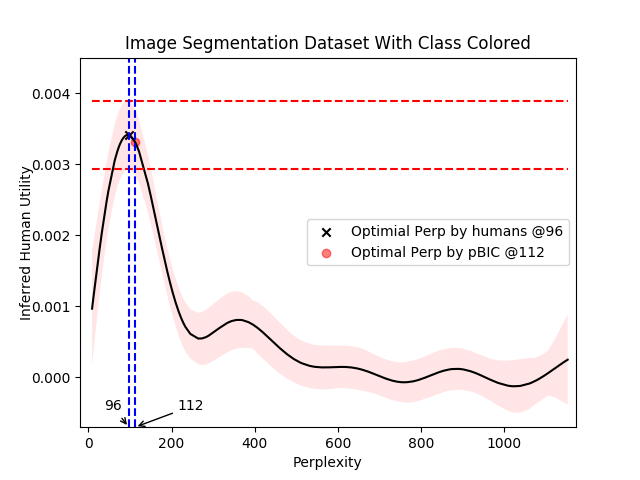} 
  \end{subfigure}  
  \begin{subfigure}{\label{fig:image_seg_bw}}
      \centering
  \includegraphics[width=2.6in]{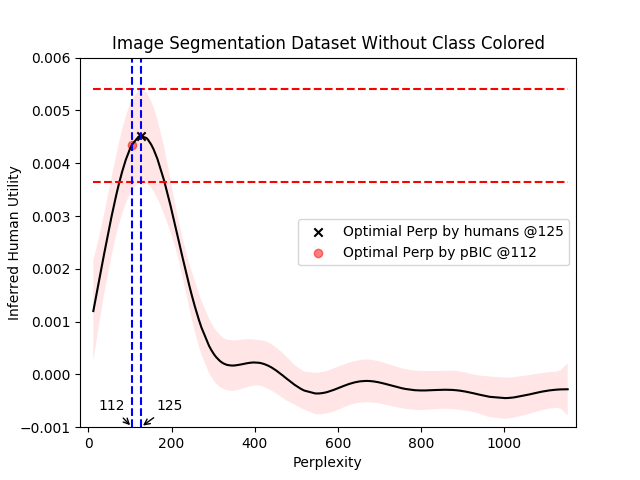}
  \end{subfigure}

  \begin{subfigure}{\label{fig:cardio_cl}}
      \centering
  \includegraphics[width=2.6in]{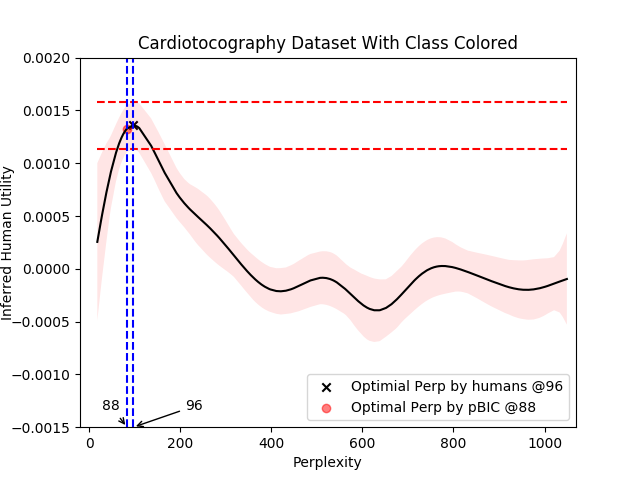}
  \end{subfigure}  
  \begin{subfigure}{\label{fig:cardio_bw}}
      \centering
  \includegraphics[width=2.6in]{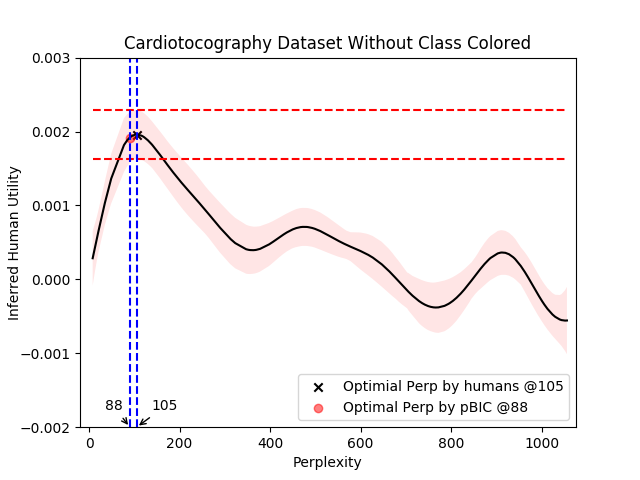}
  \end{subfigure}
  
    \begin{subfigure}{\label{fig:abalone_cl}}
      \centering
  \includegraphics[width=2.6in]{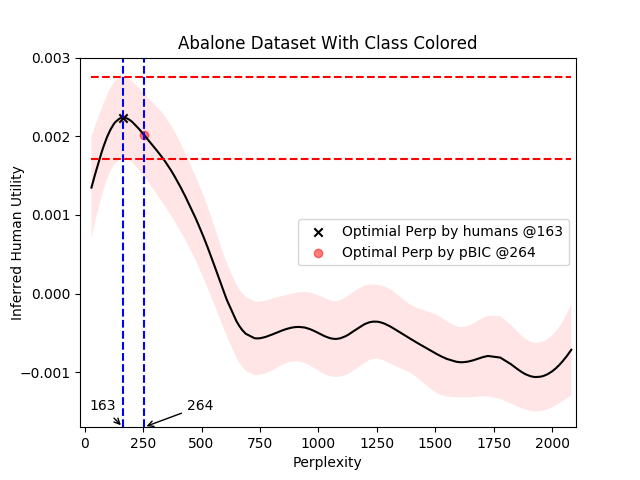}
  \end{subfigure}  
  \begin{subfigure}{\label{fig:abalone_bw}}
      \centering
  \includegraphics[width=2.6in]{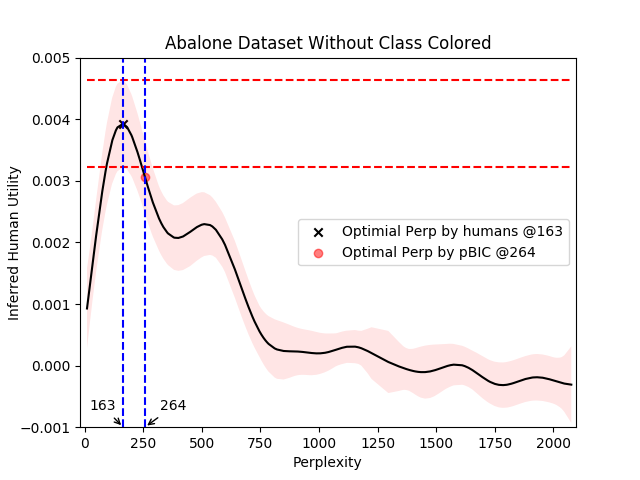}
  \end{subfigure}
  
\caption{Inferred perplexity utility functions from a single human expert on additional datasets. }
\label{main_plots}
  \end{figure}
